# Supplementary material for: ParticleSfM: Exploiting Dense Point Trajectories for Localizing Moving Cameras in the Wild
Source: arXiv:2207.09137 source file (2022-07-19)
Supplement: Supplementary file 1 [file table_supp_sintel.tex]

\begin{table}[h]
\begin{center}
\setlength{\tabcolsep}{5.0pt}
\centering
\caption{Per-scene results on MPI Sintel dataset \cite{butler2012naturalistic}.}
\begin{tabular}{clccc}
\toprule
& Methods & ATE (m) & RPE trans (m) & RPE rot (deg)\\

\midrule
\multirow{7}{*}{\textbf{alley\_2}} & COLMAP~\cite{schonberger2016structure} & 0.145 & 0.035 & 0.550\\
& MAT~\cite{zhou2020motion} +~\cite{schonberger2016structure} & 0.069 & 0.024 & 0.726\\
& Mask-RCNN~\cite{he2017mask} +~\cite{schonberger2016structure} & 0.109 & 0.039 & 0.605\\
& R-CVD~\cite{kopf2021robust} & 0.360 & 0.154 & 3.443 \\
& Tartan-VO~\cite{wang2020tartanvo} & 0.290 & 0.092 & 1.303\\
& DROID-SLAM~\cite{teed2021droid} & 0.175 & 0.084 & 1.912\\
& Ours & \textbf{0.129} & \textbf{0.031} & \textbf{0.535}\\
\midrule

\multirow{7}{*}{\textbf{alley\_2}} & COLMAP~\cite{schonberger2016structure} & 0.145 & 0.035 & 0.550\\
& MAT~\cite{zhou2020motion} +~\cite{schonberger2016structure} & 0.069 & 0.024 & 0.726\\
& Mask-RCNN~\cite{he2017mask} +~\cite{schonberger2016structure} & 0.109 & 0.039 & 0.605\\
& R-CVD~\cite{kopf2021robust} & 0.360 & 0.154 & 3.443 \\
& Tartan-VO~\cite{wang2020tartanvo} & 0.290 & 0.092 & 1.303\\
& DROID-SLAM~\cite{teed2021droid} & 0.175 & 0.084 & 1.912\\
& Ours & \textbf{0.129} & \textbf{0.031} & \textbf{0.535}\\
\midrule

\multirow{7}{*}{\textbf{alley\_2}} & COLMAP~\cite{schonberger2016structure} & 0.145 & 0.035 & 0.550\\
& MAT~\cite{zhou2020motion} +~\cite{schonberger2016structure} & 0.069 & 0.024 & 0.726\\
& Mask-RCNN~\cite{he2017mask} +~\cite{schonberger2016structure} & 0.109 & 0.039 & 0.605\\
& R-CVD~\cite{kopf2021robust} & 0.360 & 0.154 & 3.443 \\
& Tartan-VO~\cite{wang2020tartanvo} & 0.290 & 0.092 & 1.303\\
& DROID-SLAM~\cite{teed2021droid} & 0.175 & 0.084 & 1.912\\
& Ours & \textbf{0.129} & \textbf{0.031} & \textbf{0.535}\\
\midrule

\multirow{7}{*}{\textbf{alley\_2}} & COLMAP~\cite{schonberger2016structure} & 0.145 & 0.035 & 0.550\\
& MAT~\cite{zhou2020motion} +~\cite{schonberger2016structure} & 0.069 & 0.024 & 0.726\\
& Mask-RCNN~\cite{he2017mask} +~\cite{schonberger2016structure} & 0.109 & 0.039 & 0.605\\
& R-CVD~\cite{kopf2021robust} & 0.360 & 0.154 & 3.443 \\
& Tartan-VO~\cite{wang2020tartanvo} & 0.290 & 0.092 & 1.303\\
& DROID-SLAM~\cite{teed2021droid} & 0.175 & 0.084 & 1.912\\
& Ours & \textbf{0.129} & \textbf{0.031} & \textbf{0.535}\\
\midrule

\multirow{7}{*}{\textbf{alley\_2}} & COLMAP~\cite{schonberger2016structure} & 0.145 & 0.035 & 0.550\\
& MAT~\cite{zhou2020motion} +~\cite{schonberger2016structure} & 0.069 & 0.024 & 0.726\\
& Mask-RCNN~\cite{he2017mask} +~\cite{schonberger2016structure} & 0.109 & 0.039 & 0.605\\
& R-CVD~\cite{kopf2021robust} & 0.360 & 0.154 & 3.443 \\
& Tartan-VO~\cite{wang2020tartanvo} & 0.290 & 0.092 & 1.303\\
& DROID-SLAM~\cite{teed2021droid} & 0.175 & 0.084 & 1.912\\
& Ours & \textbf{0.129} & \textbf{0.031} & \textbf{0.535}\\
\midrule

\end{tabular}
\label{tab::sintel_perscene}
\end{center}
\end{table}
